# Supplementary material for: Heimdall: test-time scaling on the generative verification
Source: arXiv:2504.10337 source file (2025-04-16)
Supplement: Supplementary file 1 [file appendix.tex]

\section{Hello World}
%\subsection{Hello World}
